# Supplementary material for: Probing the shear viscosity of an active nematic
Source: arXiv:1606.05764 source file (2016-07-09)
Supplement: Supplementary file 1 [file Guillamat_etal_SI.pdf]

# Probing the shear viscosity of an active nematic

# SUPPLEMENTARY INFORMATION

Pau Guillamat[a], Jordi Ignés-Mullol[a], Suraj Shankar[b], M. Cristina Marchetti[b], and Francesc Sagués[a*]
[a]*Departament de Química Física and Institute of Nanoscience and Nanotechnology (IN2UB), Universitat de Barcelona, Martí i Franquès 1, 08028 Barcelona, Catalonia, Spain.*
[b]*Physics Department and Syracuse Soft Matter Program, Syracuse University, Syracuse, NY 13244, USA.*

## I. THE HYDRODYNAMIC MODEL: APPROXIMATIONS AND FITTING PROCEDURE

We briefly describe the solution of the hydrodynamic equations and the fitting procedure discussed in the text to obtain the defect velocity $u_0$. Assuming the flow in the nematic layer to be incompressible, the Fourier components of the flow velocity due to a force density $\mathbf{f}(\mathbf{r}) = \int_{\mathbf{k}} e^{i\mathbf{r}\cdot\mathbf{k}}\mathbf{f}(\mathbf{k})$ are given by

$$\mathbf{u}_{\perp}(\mathbf{k}) = G(k)\mathcal{P}\mathbf{f}(\mathbf{k}) \ , \tag{1}$$

where $\mathcal{P} = \boldsymbol{I} - \mathbf{k}\mathbf{k}/k^2$ is a transverse projection operator and $G(k)$ is the transverse part of the Green's function of the Stoke's equation for the nematic layer, including the coupling to the bounding fluids. The Green's function can be calculated by solving Eqs. (1-2) of the main text for the flow field in each of the three regions and imposing the incompressibility of both bulk phases. We assume that the nematic layer is an infinitely thin (compared to the two bulk layers) interface located at $z = 0$ and that the bottom aqueous phase is in contact with a no-slip wall and the oil phase has a free boundary open to air, as is appropriate for the experimental setup. By imposing continuity of tangential velocities ($\boldsymbol{u}_{i\perp} = \boldsymbol{u}_{\perp}$ at $z = 0$ for $i = o, w$) and vanishing of the normal velocity components ($\hat{\boldsymbol{n}} \cdot \boldsymbol{u}_i = 0$ at $z = 0$ for $i = o, w$), along with the continuity of normal stresses across the interface (as there is no $z$-momentum flux), we obtain

$$G(k) = \frac{1}{\eta_N k^2 + k\left[\eta_o \tanh(kd_o) + \eta_w \coth(kd_w)\right]} \ , \tag{2}$$

where $k$ is the magnitude of the in-plane wave-vector and $d_o$ and $d_w$ are the depths of the oil and water subphase layers, respectively.

We are interested in calculating the flow field due to the force distribution created by a $+1/2$ disclination located at the origin, where $\mathbf{f}(\mathbf{r}) = \alpha\boldsymbol{\nabla}\cdot\mathbf{Q}$, with [1]

$$\mathbf{Q} = S\begin{pmatrix}\cos 2\theta & \sin 2\theta \\ \sin 2\theta & -\cos 2\theta\end{pmatrix} \tag{3}$$

where $S$ is the usual scalar order parameter and $\theta$ is the angle of the director field from the $x$-axis. In polar coordinates, for a $+1/2$ defect, $\theta = \phi/2$, where $\phi$ is the polar angle, and $S = S(r)$ (taking the core to be radially symmetric) which gives

$$\mathbf{f}(\mathbf{r}) = |\alpha|\left(\frac{\mathrm{d}S}{\mathrm{d}r} + \frac{S}{r}\right)\hat{\mathbf{e}}_x \tag{4}$$

with $\hat{\mathbf{e}}_x$ being the unit vector along the $x$-axis, and $\alpha$ is the parameter related to the activity. The classical solution for $S(r) \simeq r/2\xi_Q$ vanishes linearly as $r \to 0$ ($\xi_Q$ being the core size) and tends to a constant (normalized here to unity) outside the core [2]. This allows us to approximate the only non-vanishing component of $\mathbf{f}$ as $\mathrm{f}_x = |\alpha|/\xi_Q$ for $r < \xi_Q$ and $\mathrm{f}_x = |\alpha|/r$ for $r > \xi_Q$. Finally, we assume the defect rides along with the flow and identify the defect velocity with the flow velocity created by the very distortion induced by the defect at the core of the defect, given by

$$u_0 = \int_{\mathbf{k}}' G(k)(\mathcal{P}\mathbf{f}(k))_x = \frac{1}{2}\int_{\mathbf{r}}' G(r)\mathrm{f}_x(r) \ , \tag{5}$$

*Electronic address: f.sagues@ub.edu

where the prime denotes suitable large and small scale cutoffs and we have used the fact that both $G(r)$ and $\mathrm{f}_x(r)$ are independent of the polar angle resulting in the angular average of the projection operator $\mathcal{P}$ which gives a factor of 1/2.

Evaluating Eq. (5) exactly is challenging. For this reason we take advantage of the fact that when $d_w \sim d_o \sim d$ are large, both $\tanh(kd)$ and $\coth(kd)$ are approximately unity. Neglecting $\eta_w$ compared to $\eta_o$ (as $\eta_w \ll \eta_o$), we then obtain the approximate expression

$$G(k) \simeq G_>(k) = \frac{1}{\eta_N k^2 + \eta_o k} \ , \quad \text{for} \ \ kd \gg 1 \ , \tag{6}$$

$$G(k) \simeq G_<(k) = \frac{1}{(\eta_N + \eta_o d)k^2 + \eta_w/d} = \frac{1}{\eta_R(k^2 + \ell_\Gamma^{-2})} \ , \quad \text{for} \ \ kd \ll 1 \ , \tag{7}$$

where $\ell_\Gamma = \sqrt{\eta_R d/\eta_w}$ is the frictional screening length and $\eta_R = \eta_N + \eta_o d$ is a renormalized $2d$ nematic viscosity. Note that even for $kd = 2$, we only have about 4% error in using the approximation $G(k) \simeq G_>(k)$ that replaces the hyperbolic functions by unity. We expect $\ell_\Gamma > d$ and $\eta_R \simeq \eta_N$, both of which will be verified a posteriori.

We compute the disclination core velocity from Eq. (5) by evaluating the integral in real space and cutting it off at small scales with the defect core size $\xi_Q$ (below which we do not expect the hydrodynamic description to remain valid) and at large scales by the lateral system size $L$, with the result

$$u_0 = u_< + u_> \ , \tag{8}$$

$$u_< = \frac{1}{2}\int_d^L \mathrm{d}^2 r \ G_<(r)\frac{|\alpha|}{r} = \frac{|\alpha|\ell_\Gamma}{\eta_R}\mathcal{F}_<\left(\frac{L}{\ell_\Gamma}, \frac{d}{\ell_\Gamma}\right) \tag{9}$$

$$u_> = \frac{1}{2}\int_{\xi_Q}^d \mathrm{d}^2 r \ G_>(r)\frac{|\alpha|}{r} = \frac{|\alpha| d}{\eta_N} \ \mathcal{F}_>\left(\frac{\eta_o d}{\eta_N}, \frac{d}{\xi_Q}\right) \ , \tag{10}$$

The general scaling functions $\mathcal{F}_>$ and $\mathcal{F}_<$ are given by

$$\mathcal{F}_<\left(\frac{L}{\ell_\Gamma}, \frac{d}{\ell_\Gamma}\right) = \int_{d/\ell_\Gamma}^{L/\ell_\Gamma} \mathrm{d}x \ K_0(x) \ , \tag{11}$$

$$\mathcal{F}_>\left(\frac{\eta_o d}{\eta_N}, \frac{d}{\xi_Q}\right) = \frac{\pi}{2}\int_{\xi_Q/d}^1 \mathrm{d}x \left[\mathbb{H}_0\left(\frac{\eta_o d}{\eta_N}x\right) - Y_0\left(\frac{\eta_o d}{\eta_N}x\right)\right] \ , \tag{12}$$

with $K_n(x)$ and $Y_n(x)$, the (modified) Bessel functions and $\mathbb{H}_n(x)$ the Struve function.

In the limit $\eta_o d/\eta_N \ll 1$ and $d/\xi_Q \gg 1$, the expressions for $u_<$ and $u_>$ simplify to give

$$u_< \simeq \frac{|\alpha|\ell_\Gamma}{\eta_N}\mathcal{F}_<\left(\frac{L}{\ell_\Gamma}, \frac{d}{\ell_\Gamma}\right) \ , \tag{13}$$

$$u_> \simeq \frac{|\alpha| d}{\eta_N}\left\{1 + \ln\left(\frac{2\eta_N}{\eta_o d}\right) - \frac{\xi_Q}{d}\left[1 + \ln\left(\frac{2\eta_N}{\eta_o \xi_Q}\right)\right]\right\} \ , \tag{14}$$

where we have only retained the leading order terms in Eq. (14). The only change in the expression for $u_<$ in Eq. (13) is that it is now approximately independent of the oil viscosity, as $\eta_R \approx \eta_N$ (as $\eta_o d \ll \eta_N$) and consequently $\ell_\Gamma \approx \sqrt{\eta_N d/\eta_w}$, leaving $u_<$ as a constant.

In the experimental setup $L \sim 2.5$ mm and $d \sim 1$ mm are of the same magnitude. Using $L/\ell_\Gamma \sim d/\ell_\Gamma \ll 1$ we simplify Eq. (13) further to

$$u_< \simeq \frac{|\alpha|(L-d)}{\eta_N}\ln\left(\frac{2\ell_\Gamma}{d}\right) \ , \tag{15}$$

which shows that $u_<$ is very small and approximately independent of the oil viscosity for our purposes. Hence the defect speed is determined by $u_>$ and its dominant contribution for $\eta_N/d \gg \eta_o$ is given by

$$u_0 \sim \frac{|\alpha| d}{\eta_N}\ln\left(\frac{\eta_N}{\eta_o d}\right) \ . \tag{16}$$

The same behavior can be obtained by evaluating $u_>$ by approximating the Green's function $G_>(r)$ for $r \ll \ell_\eta$, with $\ell_\eta = \eta_N/\eta_o$, as

$$G_>(r) \simeq \frac{1}{2\pi\eta_N}\ln\left(1 + \frac{\ell_\eta}{r}\right) \ , \tag{17}$$

Evaluating the integral using this approximate form of $G_>$, we immediately get Eq. (14) (upto factors of 2 present in the logarithm). Hence, as mentioned in the main text, the logarithmic dependence comes essentially because the flow is primarily two-dimensional (due to the high nematic viscosity), with the oil only entering as a logarithmic correction to the length scale of the velocity. The validity of this approximation is verified a posteriori by fitting to the experimental results. Note that if we instead assume $r \gg \ell_\eta$, then $G_>(r) \sim 1/(\eta_o r)$, which will always give rise to a $1/\eta_o$ dependence of $u_0$ on the oil viscosity, much stronger than the logarithmic one seen in the experiments.

We have fitted the experimental data using both the approximate expression for $u_0$ given in Eq. (16) and the more complete expression using Eq. (8 - 12), and find $\eta_N \sim 42 \times 10^{-3}$ Pa s m and $\eta_N = 13(\pm 5) \times 10^{-3}$ Pa s m, respectively. Using $d = 1$ mm, both values satisfy the condition $\eta_N \gg \eta_o d$ for all but the largest value of $\eta_o$, justifying our approximations. A comparison of the two fits is shown in Fig. (1). The inset of this figure shows that the fitted value depends weakly on the cutoff $\xi_Q/d$, provided $\xi_Q/d < 0.5$. The overall velocity scale also determines the activity, yielding $|\alpha| = 1 - 10 \times 10^{-5}$ Pa m. Dividing by the thickness of the active nematic layer ($\sim 0.2\mu$m $- 2\mu$m), we find the activity to be $\sim 50 - 500$ Pa, which is in the range of the active stress estimated for cytoskeletal acto-myosin networks [3–5].

Finally, it is clear that while the logarithmic dependence on $u_0$ on oil viscosity and the fitted value of the effective three-dimensional viscosity $\eta_N/d$ are robust, the value of $\eta_N$ itself depends on the long-wavelength cutoff used in the integration, here chosen as $d$.

In fact one could argue that the the single-defect calculation described above is not appropriate for the system of interest that contains many defects. In this case as the nematic order parameter rapidly goes to zero beyond the mean inter-defect separation, a more suitable cutoff would be the mean defect separation $\ell_\mathrm{d} = n^{-1/2}$, where $n$ is the defect number density, with $\ell_\mathrm{d} < d$. In this case $\mathbf{f}(\mathbf{r})$ will vanish for $r > \ell_\mathrm{d}$, so that $u_0$ is given entirely by $u_>$, with the replacement $d \to \ell_\mathrm{d}$ for the upper cutoff, with the result

$$u_0 \simeq \frac{|\alpha|\ell_\mathrm{d}}{\eta_N}\mathcal{F}_>\left(\frac{\eta_o\ell_\mathrm{d}}{\eta_N}, \frac{\ell_\mathrm{d}}{\xi_Q}\right) \sim \frac{|\alpha|\ell_\mathrm{d}}{\eta_N}\ln\left(\frac{\eta_N}{\eta_o\ell_\mathrm{d}}\right) , \tag{18}$$

where the last approximate equality holds for $\eta_o\ell_\mathrm{d}/\eta_N \ll 1$.

In summary, the hydrodynamic calculation requires a long-wavelength cutoff arising from the screening of the $2d$ hydrodynamic flows by the confining bulk layers. Provided this cutoff exceeds the short-wavelength cutoff $\xi_Q$ and is smaller than the lateral system size, the main contribution to the defect velocity comes from $u_>$ alone. Denoting generically this long-wavelength cutoff by $\ell$, we find that if $\eta_N/\ell \gg \eta_o$, the hydrodynamic theory predicts the logarithmic dependence of the defect velocity on oil viscosity seen in experiments, with

$$u_0 \simeq\sim \frac{|\alpha|\ell}{\eta_N}\ln\left(\frac{\eta_N}{\eta_o\ell}\right) , \tag{19}$$

as given in the main text. Furthermore, a fit of the data provides a robust value for the effective bulk viscosity $\eta_\mathrm{eff} = \eta_N/\ell$ of the active nematic, largely independent of $\ell$ (see inset of Fig. 1). The fitted value satisfies the assumption $\eta_N/\ell \gg \eta_o$ at all but the largest value of oil viscosity used in the experiments, where the defect velocity saturates. The value of the $2d$ nematic viscosity $\eta_N$ is of course sensitive to the value of $\ell$, as discussed in the main text.

## II. SUPPLEMENTARY FIGURES

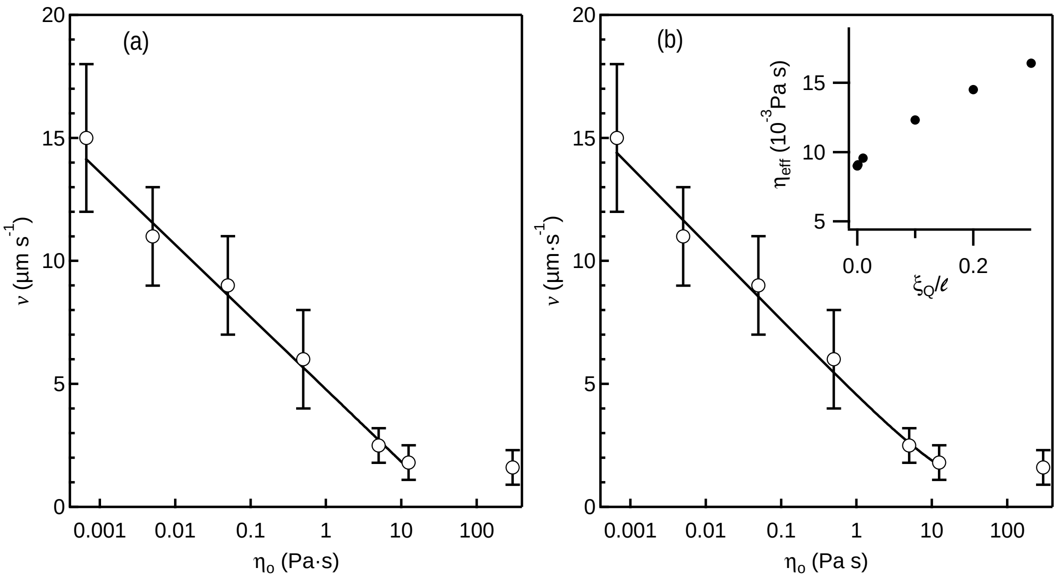


FIG. 1: Comparison of the approximate (a) and exact (b) fit of the velocity vs. viscosity data using the model described in the text.The inset includes the effective bulk viscosity $\eta_{\text{eff}} = \eta_N/\ell$ obtained from the fit using Eq. (8 - 12), as a function of the ratio between the defect core size $\xi_Q$ and the cutoff length scale $\ell$.

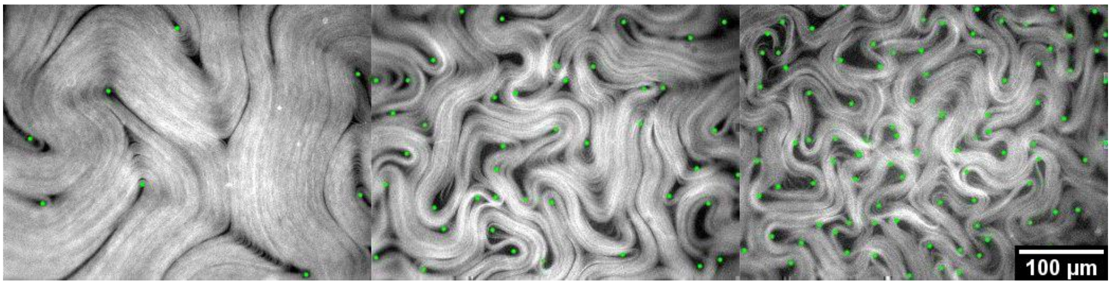


FIG. 2: Changes in the morphology and dynamics of an active nematic bounded by oils of different viscosity. Fluorescence micrographs of the active nematic show an increase in the number of defects and a decrease of their speed with increasing oil viscosity: 0.05, 5 and 300 Pa s from left to right. The green spots indicate the location of the +1/2 defects (VideoS1.mov).

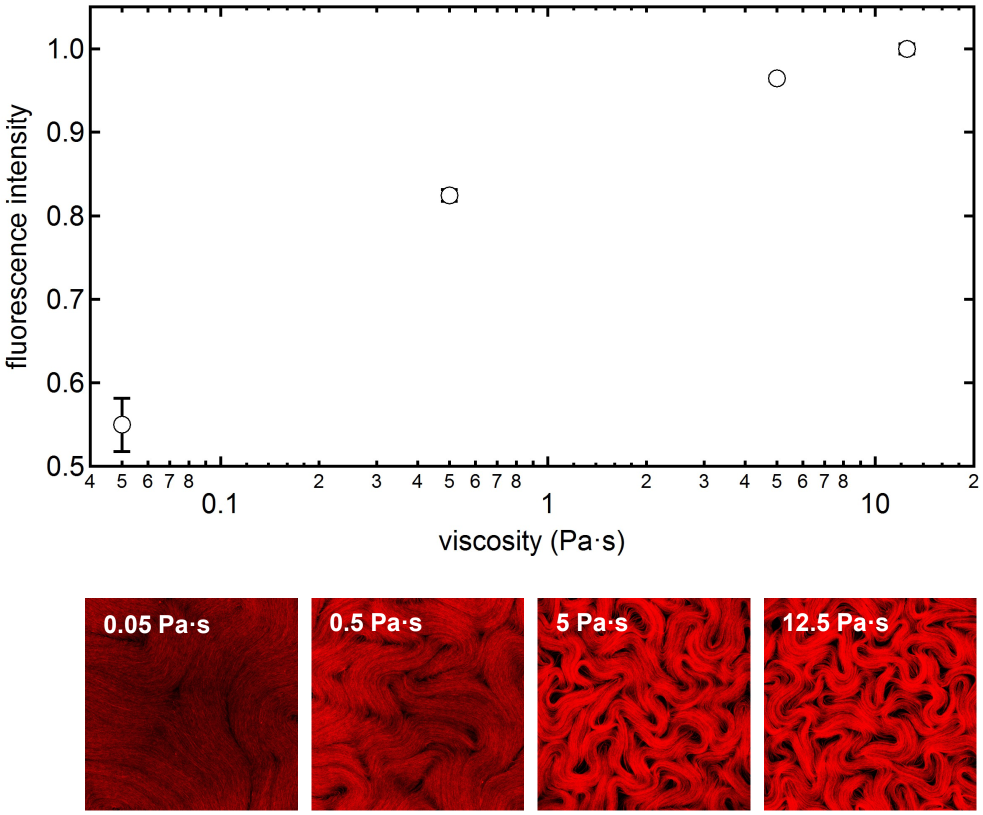


FIG. 3: Average fluorescence intensity of the active nematic in contact with oils of different viscosity. The data have been obtained with confocal fluorescence microscopy maintaining constant values of all imaging parameters.

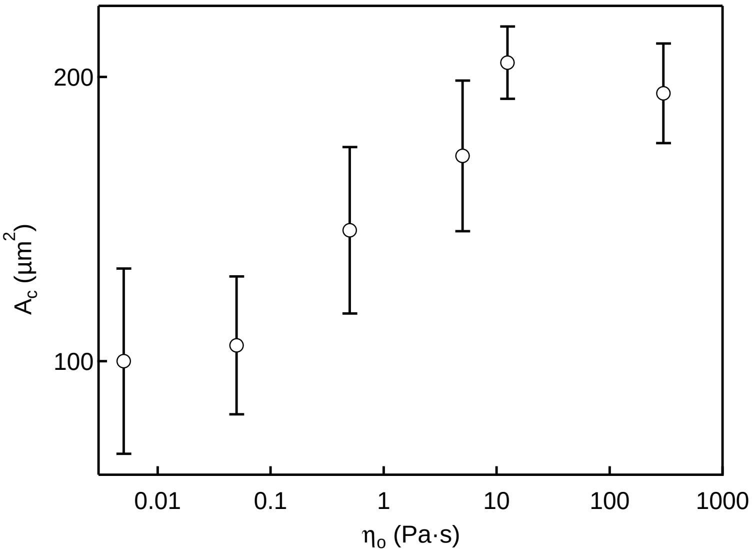


FIG. 4: Average area of the defect core as a function of contacting oil viscosity. The area has been obtainined from confocal fluorescence micrographs by measuring the total area devoid of fluorescent material surrounding each defect in a given region of the micrograph, and dividing it by the number of defects in the same region.

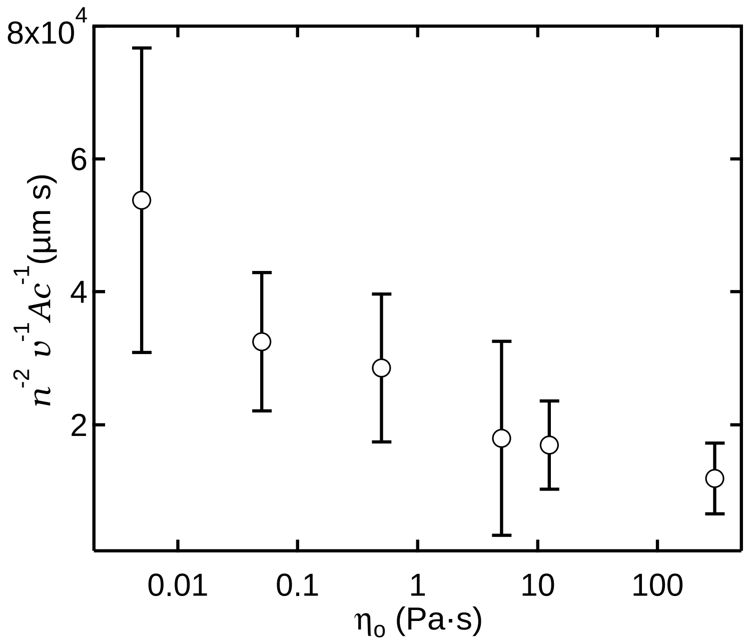


FIG. 5: Scaling of the defect velocity, number density, and core area with oil viscosity. Assuming $K \sim \xi_Q^2 \sim A_c$, the scaling argument based on the rate equation for defects discussed in the main text predicts that for fixed activity $n^{-2}\ v^{-1} A_c^{-1} \sim \gamma\sigma$. Assuming $\gamma$ does not depend on oil viscosity, the figure then shows that the defect cross section $\sigma$ decreases with oil viscosity, suggesting that this length scale does not coincide with the defect core size $\xi_Q$ that is observed to increase with $\eta_o$.


[1] L. M. Pismen, Phys Rev E Stat Nonlin Soft Matter Phys **88**, 050502 (2013).

[2] L. M. Pismen, *Vortices in nonlinear fields: From liquid crystals to superfluids, from non-equilibrium patterns to cosmic strings*, vol. 100 (Oxford University Press, 1999).

[3] K. Kruse, J. Joanny, F. Jülicher, and J. Prost, Physical biology **3**, 130 (2006).

[4] G. Salbreux, J. Prost, and J.-F. Joanny, Physical review letters **103**, 058102 (2009).

[5] J. Prost, F. Jülicher, and J. Joanny, Nature Physics **11**, 111 (2015).
